# Supplementary material for: Enhancing Efficiency in Vision Transformer Networks: Design Techniques and Insights
Source: arXiv:2403.19882 source file (2024-03-28)
Supplement: Supplementary file 1 [file appendix.tex]

% \subsection*{Availability of data and materials}
% All data used in this study are publicly available.

\subsection*{Funding}
This work was funded by the German Research Foundation (Deutsche Forschungsgemeinschaft, DFG) under project numbers 191948804, 527820737 and 455548460.

\subsection*{Declaration of competing interest}
The authors have no competing interests to declare relevant to this article's content.

\subsection*{Authors' contributions}
RA designed the study concept and the evaluation, and contributed to writing. MD and NK contributed to the writing. DM revised the study concept. All authors reviewed the manuscript.
